# Supplementary material for: Vacancy-free cubic superconducting NbN enabled by quantum anharmonicity
Source: arXiv:2507.03417 source file (2025-07-04)
Supplement: Supplementary file 1 [file Suppl.pdf]

# SUPPLEMENTARY INFORMATION

## ‘Vacancy-free cubic superconducting NbN enabled by quantum anharmonicity’

Eva Kogler,[1] Mihir R. Sahoo,[1] Chia-Nien Tsai,[2] Fabian Jöbstl,[1] Roman Lucrezi,[1,3] Peter I. C. Cooke,[4] Birgit Kunert,[5] Roland Resel,[5] Chris J. Pickard,[4,6] Matthew N. Julian,[7] Rohit P. Prasankumar,[7] Mahmoud I. Hussein,[8,2] and Christoph Heil[1,*]

[1]*Institute of Theoretical and Computational Physics, Graz University of Technology, NAWI Graz, 8010, Graz, Austria*

[2]*Smead Department of Aerospace Engineering Sciences, University of Colorado, Boulder, Colorado 80303*

[3]*Department of Materials and Environmental Chemistry, Stockholm University, SE-10691 Stockholm, Sweden*

[4]*Department of Materials Science and Metallurgy, University of Cambridge, 27 Charles Babbage Road, Cambridge, CB3 0FS, UK*

[5]*Institute of Solid State Physics, Graz University of Technology, NAWI Graz, 8010, Graz, Austria*

[6]*Advanced Institute for Materials Research, Tohoku University, Sendai, 980-8577, Japan*

[7]*Intellectual Ventures, Bellevue, Washington, United States*

[8]*Department of Physics, University of Colorado, Boulder, Colorado 80302*

(Dated: July 4, 2025)

* Corresponding author: christoph.heil@tugraz.at

## S1. $P\bar{4}3m$ structural details

A cubic structure with space group P$\bar{4}$3m (215) and lattice parameter of $a = 4.421$ Å is identified. Niobium and nitrogen atoms occupy the 4e Wyckoff positions with fractional coordinates x=0.732 and 0.234, respectively, forming a non-centrosymmetric, vacancy-free cubic phase.

## S2. Total energies of various NbN phases

Table S1: Energy comparison of various NbN structures. Only phases with a (close to) 1:1 ratio are considered. $\Delta E_{\mathrm{el}}$ is the electronic total energy and $\Delta G$ is the free energy including the zero point energy. Both are given with respect to the corresponding value of the $P\bar{4}3m$ SSCHA structure.

| Label | Symmetry | $\Delta E_{\mathrm{el}}$ (meV/atom) | $\Delta G$ (meV/atom) |
|---|---|---|---|
| $\delta$ (small smearing) | $Fm\bar{3}m$ | 37 | – |
| $\delta$ (large smearing) | $Fm\bar{3}m$ | 68 | 65 |
| $\delta'$ | $P6_3/mmc$ | -118 | -107 |
| $\epsilon$ | $P6_3/mmc$ | -141 | -130 |
| $\epsilon'$ | $P6_3/mmc$ | 53 | 53 |
| NbO-like | $Pm\bar{3}m$ | 389 | 381 |

Table S2: Calculated enthalpies ($\Delta H$) and pressures ($P$) of the lowest-enthalpy NbN phases identified by AIRSS. A high-symmetry search (2–48 symmetry operations) using ephemeral data-derived potentials (EDDPs) sampled $\sim$ 50,000 structures in 64-atom (1:1 Nb:N) cells. The lowest-enthalpy candidates were subsequently refined by high-quality DFT relaxations and hexagonal structures were removed. $\Delta H$ is given relative to $P\bar{4}3m$; $P$ is in GPa; and $f.u.$ denotes the number of formula units per cell.

| Structure ID | Crystal system | Symmetry | $f.u.$ | $\Delta H$ (meV/f.u.) | $P$ (GPa) | $V$ (Å$^3$) |
|---|---|---|---|---|---|---|
| NbN-1410118-4002-233 | cubic | $P\bar{4}3m$ | 4 | -1935.252 | 0.07 | 21.579 |
| NbN-3916838-1730-38 | tetragonal | $P4_2/mcm$ | 4 | 2 | -0.00 | 21.600 |
| NbN-2008120-7812-127 | orthorhombic | $Ibam$ | 8 | 3 | -0.05 | 21.610 |
| NbN-3916842-1904-379 | tetragonal | $P4/nmm$ | 2 | 4 | 0.00 | 21.607 |
| NbN-1410113-208-318 | orthorhombic | $Pmma$ | 8 | 31 | 0.00 | 21.587 |
| NbN-2008101-5566-498 | trigonal | $P\bar{3}$ | 32 | 34 | -0.02 | 23.051 |
| NbN-3916827-7102-465 | tetragonal | $P4_2/mcm$ | 16 | 36 | -0.01 | 21.593 |
| NbN-323863-7025-457 | tetragonal | $P4_2/mcm$ | 16 | 36 | -0.00 | 21.594 |
| NbN-1410131-467-11 | orthorhombic | $Pbca$ | 32 | 120 | -0.01 | 23.287 |

Table S3: Calculated enthalpies ($\Delta H$) and pressures ($P$) of the lowest-enthalpy NbN structures identified by relaxation of shaken *fcc* supercells comprising 2-6 formula units of NbN.

| Structure ID | Crystal system | Symmetry | *f.u.* | $\Delta H$ (meV/f.u.) | $P$ (GPa) | $V$ (Å$^3$) |
|---|---|---|---|---|---|---|
| NbN-830789-1698-8 | cubic | $P\bar{4}3m$ | 4 | -1935.252 | -0.04 | 21.593 |
| NbN-984511-9845-1 | orthorhombic | $Ibam$ | 4 | 1 | 0.03 | 21.618 |
| NbN-474547-5399-7 | tetragonal | $P4/nmm$ | 2 | 4 | 0.01 | 21.604 |
| NbN-1523477-3927-9 | tetragonal | $I\bar{4}2m$ | 4 | 6 | 0.02 | 21.608 |
| NbN-680767-3732-7 | monoclinic | $C2/m$ | 2 | 7 | -0.03 | 21.607 |
| NbN-2266156-5849-8 | monoclinic | $C2/m$ | 2 | 8 | -0.03 | 21.609 |
| NbN-464903-1830-6 | triclinic | $P1$ | 5 | 22 | 0.03 | 21.622 |
| NbN-474547-5399-5 | monoclinic | $Cm$ | 5 | 22 | -0.08 | 21.627 |
| NbN-2417718-1018-4 | triclinic | $P\bar{1}$ | 5 | 23 | 0.01 | 21.618 |
| NbN-451827-380-9 | monoclinic | $Cc$ | 6 | 28 | -0.01 | 21.638 |
| NbN-2990131-3476-1 | orthorhombic | $Imm2$ | 3 | 35 | -0.03 | 21.602 |
| NbN-830797-3694-5 | triclinic | $P\bar{1}$ | 5 | 35 | 0.00 | 21.631 |
| NbN-464901-2130-14 | monoclinic | $C2/m$ | 3 | 36 | 0.02 | 21.593 |
| NbN-2266154-5824-10 | tetragonal | $I\bar{4}$ | 5 | 38 | 0.05 | 21.641 |
| NbN-1523471-3886-5 | monoclinic | $C2$ | 6 | 43 | -0.01 | 21.672 |
| NbN-925057-730-10 | monoclinic | $C2$ | 6 | 44 | 0.00 | 21.671 |
| NbN-2396524-2467-5 | triclinic | $P\bar{1}$ | 6 | 46 | 0.03 | 21.660 |
| NbN-2077963-2685-6 | monoclinic | $C2/m$ | 4 | 64 | -0.03 | 21.680 |
| NbN-460234-513-11 | monoclinic | $C2$ | 5 | 65 | -0.04 | 21.624 |
| NbN-474545-5381-8 | monoclinic | $C2/m$ | 5 | 66 | 0.06 | 21.668 |
| NbN-2990139-3566-7 | monoclinic | $C2/m$ | 5 | 67 | 0.03 | 21.669 |
| NbN-437928-1290-10 | triclinic | $P\bar{1}$ | 4 | 73 | -0.00 | 21.657 |
| NbN-464895-973-6 | cubic | $Fm\bar{3}m$ | 1 | 78 | 0.04 | 21.596 |

## S3. Electronic dispersions

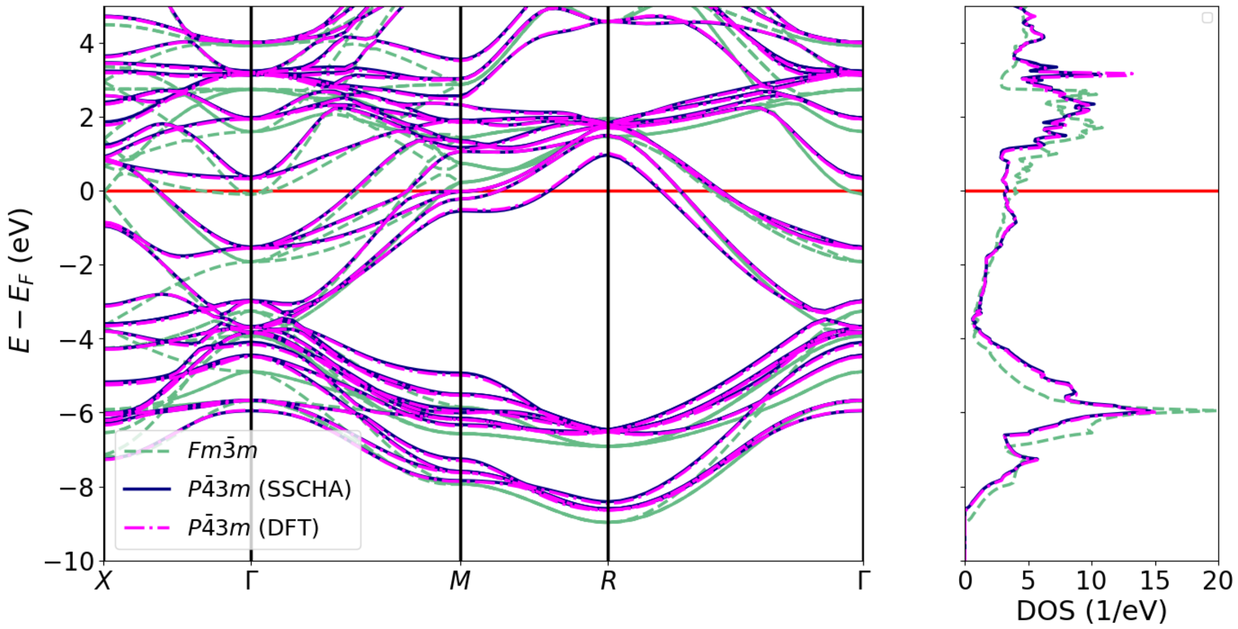


Figure S1: Electronic dispersion (left panel) and DOS (right panel) of the $Fm\bar{3}m$ (dashed green) and the $P\bar{4}3m$ structure - DFT relaxed (dash-dotted magenta) and SSCHA relaxed (solid blue).

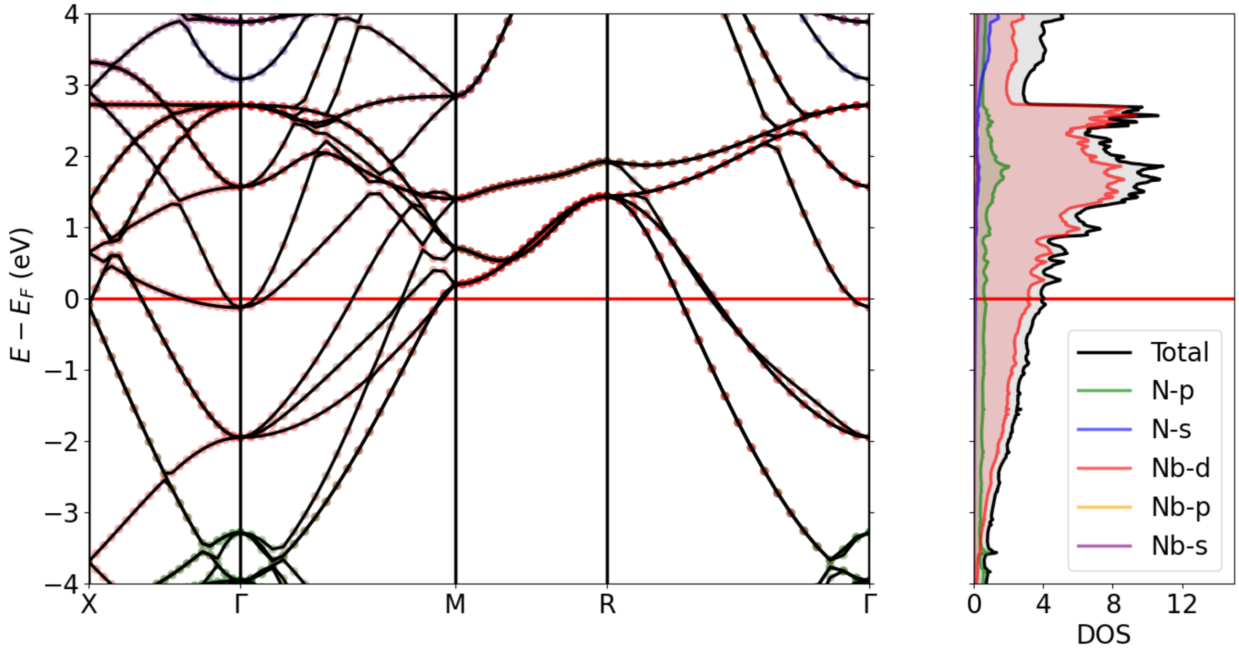


Figure S2: Electronic dispersion (left panel), and DOS (right panel) of the $Fm\bar{3}m$ structure. The projected DOS includes contributions from Nb-$s$, $p$, and $d$, as well as N-$s$ and $p$ orbitals. Orbital character projections are also indicated in the band structure.

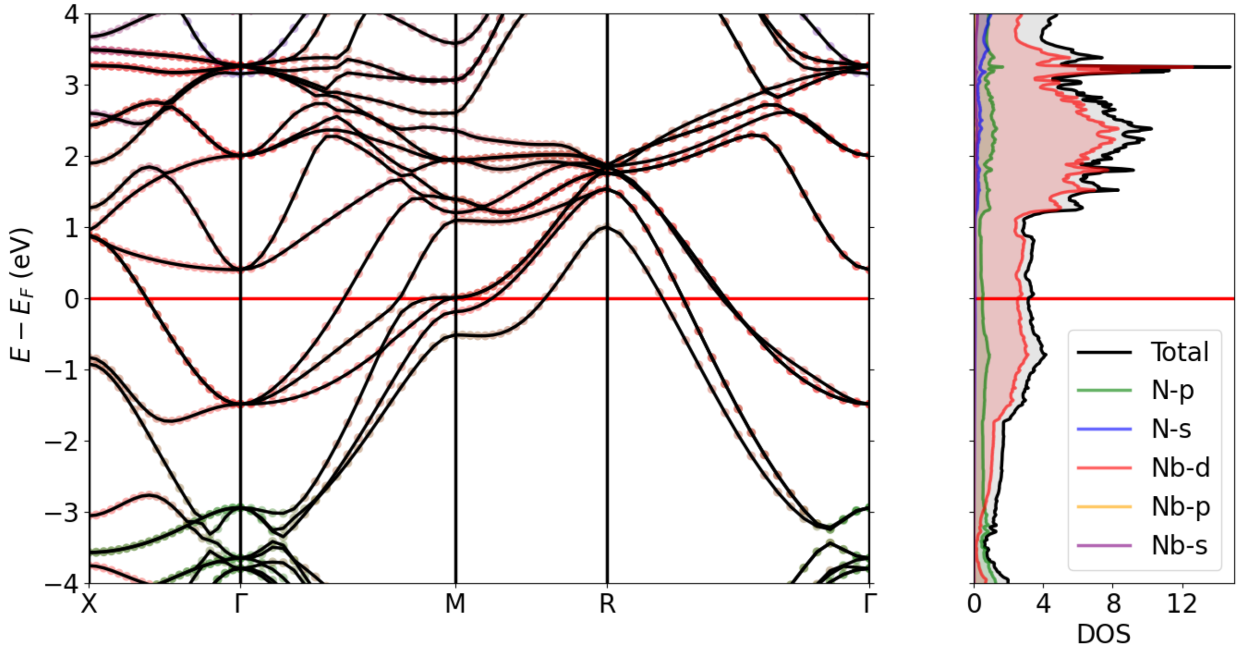


Figure S3: Electronic dispersion (left panel), and DOS (right panel) of the $P\bar{4}3m$ structure. The projected DOS includes contributions from Nb-$s$, $p$, and $d$, as well as N-$s$ and $p$ orbitals. Orbital character projections are also indicated in the band structure.

## S4. Phononic dispersions

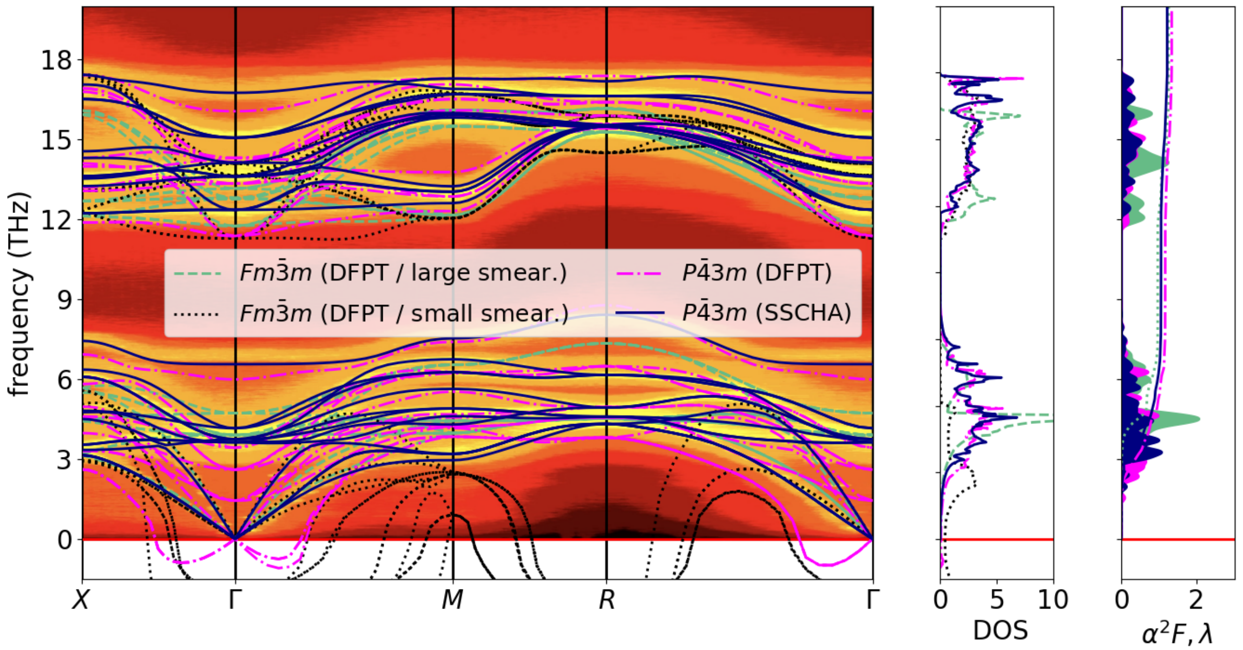


Figure S4: Phonon dispersion (left panel), phonon DOS (middle panel), and $\alpha^2F$ and $\lambda$ (right panel) in the harmonic approximation of the $Fm\bar{3}m$ with large smearing (dashed green) and small smearing (dotted black) the $P\bar{4}3m$ structure (dash-dotted magenta), and of the $P\bar{4}3m$ structure within SSCHA at 15 K (solid blue) for a $4 \times 4 \times 4$ phonon grid. The spectral information in the background has been obtained with SED.

## S5. Fermi surface resolved orbital character and $\lambda$

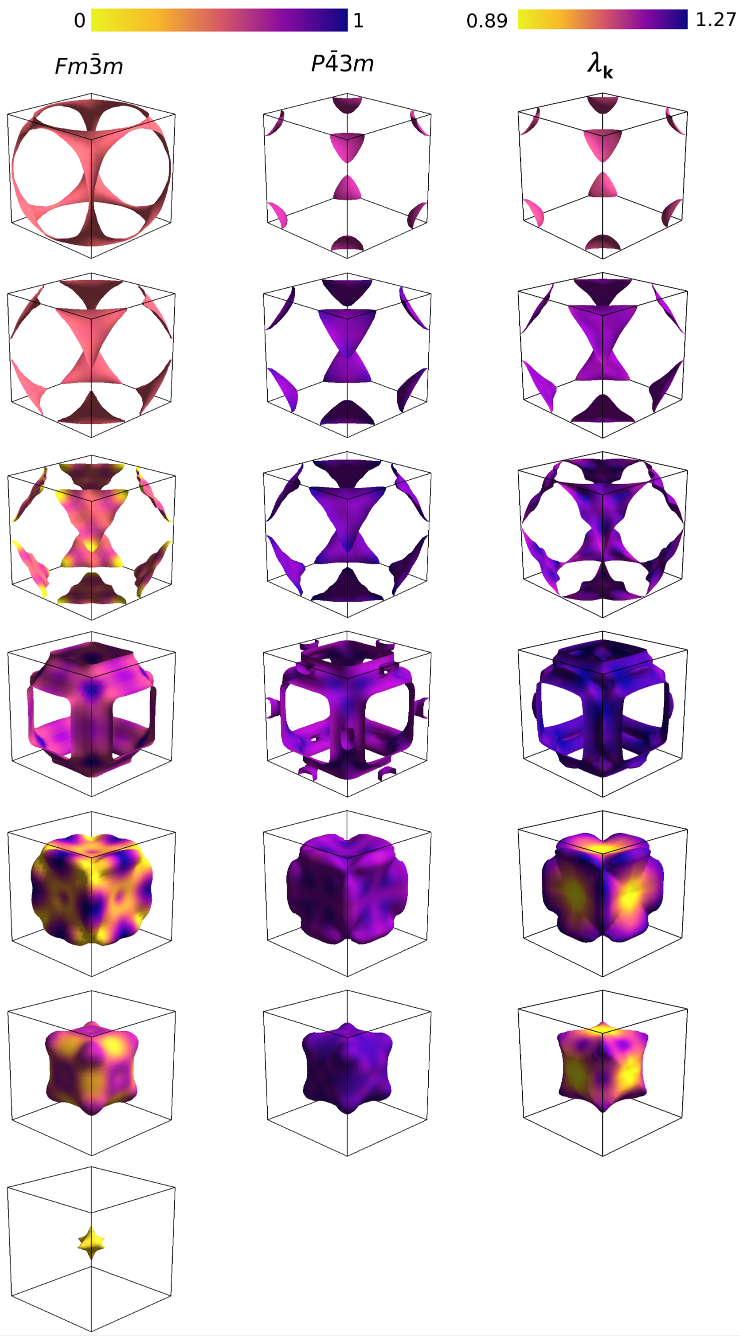


Figure S5: Fermi surface broken down into single bands for the $Fm\bar{3}m$ (left column) and $P\bar{4}3m$ (middle and right column) structure. The first two columns are colored by the Nb $d$-orbital character from yellow (0) to blue (1). The right column is colored by $\lambda_{\mathbf{k}}$ from an anisotropic ME calculation.

## S6. Details on SSCHA calculations for NbC and TiN

We applied the same SSCHA relaxation procedure described in the main text to TiN and NbC. As shown in Fig. S6 and Fig. S7, the symmetry of the initial $Fm\bar{3}m$ structures remained unchanged. This outcome is consistent with the fact that TiN and NbC are already dynamically stable and suggests that, unlike NbN, quantum ionic motion and anharmonic effects do not drive a structural instability in these materials.

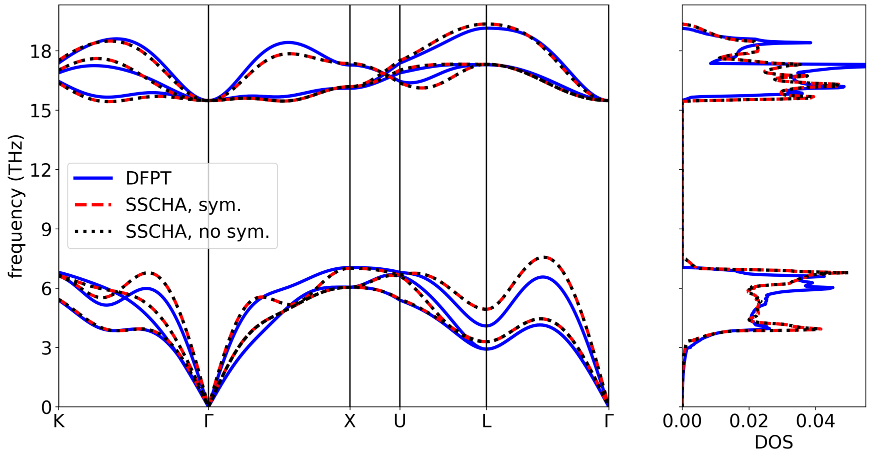


Figure S6: Comparison of phonon dispersions (left panel) and phonon densities of states (right panel) for NbC, obtained from DFPT (solid blue), SSCHA with enforced symmetry (dashed red, SSCHA, sym.), and SSCHA with full structural relaxation (dotted black, SSCHA, no sym.). The two SSCHA calculations yield identical results, indicating that full structural relaxation does not lead to symmetry lowering.

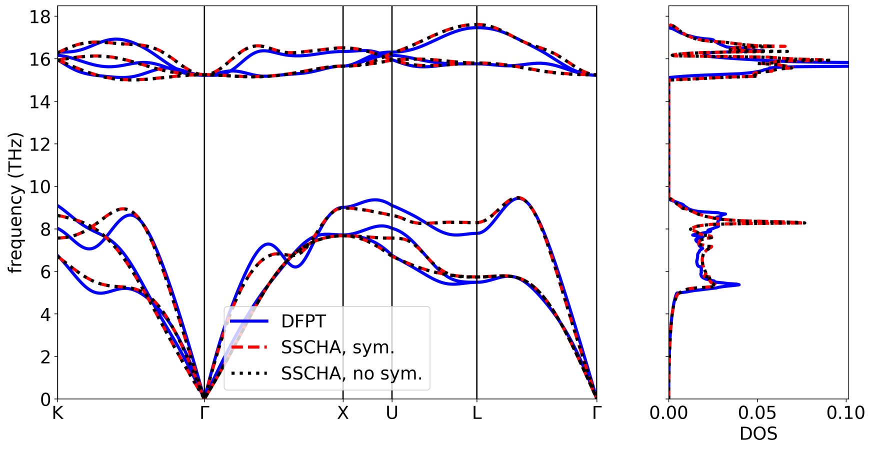


Figure S7: Comparison of phonon dispersions (left panel) and phonon densities of states (right panel) for TiN, obtained from DFPT (solid blue), SSCHA with enforced symmetry (dashed red, SSCHA, sym.), and SSCHA with full structural relaxation (dotted black, SSCHA, no sym.). The two SSCHA calculations yield identical results, indicating that full structural relaxation does not lead to symmetry lowering.

## S7. MTP validation

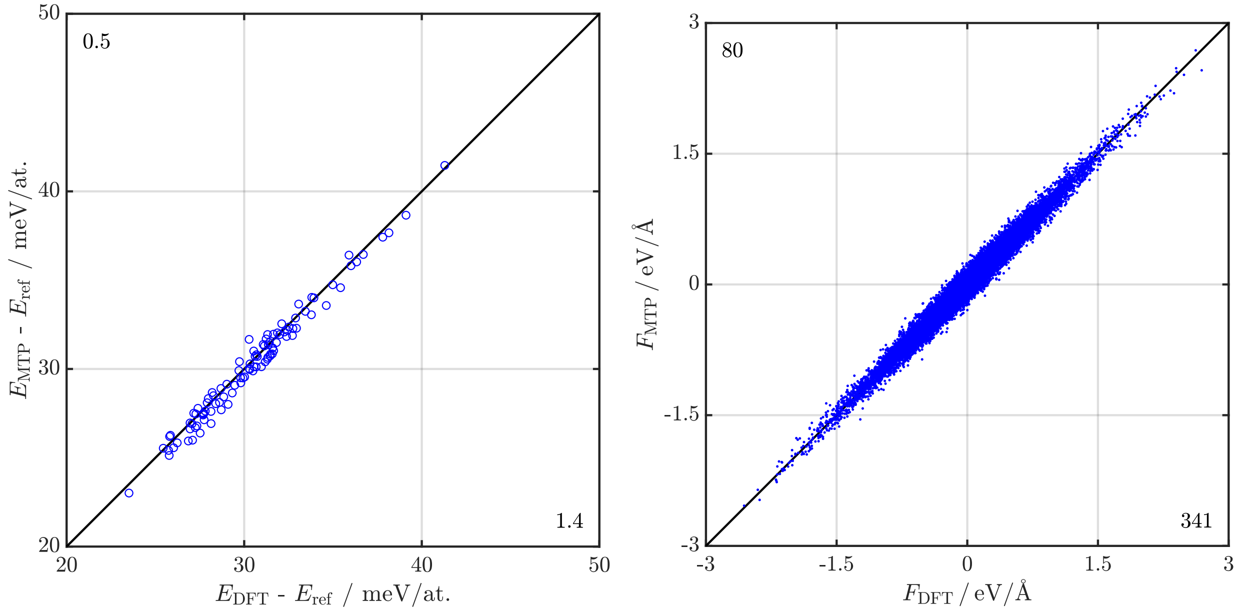


Figure S8: MTP validation for the $P\bar{4}3m$ structure in a 2×2×2 supercell containing 64 atoms. Energy ($E$) and force components ($F$) correspond to a random set of 100 structures out of the last (converged and relaxed) SSCHA population at 15 K without any symmetry constraints. The MTP values for these structures are plotted versus the corresponding DFT values. The energies are plotted with respect to the DFT total energy of the $P\bar{4}3m$ structure $E_{\mathrm{ref}}$. The solid black line indicating the perfect correlation between MTP and DFT values serves as a guide to the eye. The values at the top left indicate the RMSE and at the bottom right the maximum absolute difference in units of meV (meV/Å) for $E$ ($F$).

## S8. Details on the SED calculations

The SED method allows us to obtain the phonon band structure directly from equilibrium molecular dynamics simulations where anharmonic effects are fully accounted for. This method consists of two main steps. First, MD simulations are performed using the LAMMPS [S1], during which the velocity of each atom is recorded over time. Second, in the post-processing stage, a Fourier transform is applied to the recorded velocity data to generate the SED spectrum, which provides a frequency-versus-wavenumber mapping of the phonon energy distribution. In this work, the SED approach requires only the crystal unit-cell structure and does not require any prior knowledge of phonon mode eigenvectors.

The MD model is based on a cubic NbN unit cell with a lattice parameter of $a$ = 4.482262 Å. As illustrated in Fig. S9, the unit cell contains 4 niobium (Nb) and 4 nitrogen (N) atoms. A supercell is composed of $N = N_x \times N_y \times N_z = 30 \times 30 \times 30$ unit cells, forming the total simulated computational domain. Periodic boundary conditions are applied along all three directions. The use of a large supercell is essential for resolving phonon modes propagating in multiple directions. The system is first equilibrated under the $NPT$ ensemble

at 16 K for 0.2 ns. After equilibration, the ensemble is switched to the $NVE$ for velocity data collection. The system is simulated for $2^{20}$ time steps with a time interval of $\Delta t = 0.5$ fs. Velocity data are extracted every $2^5$ steps for SED analysis.

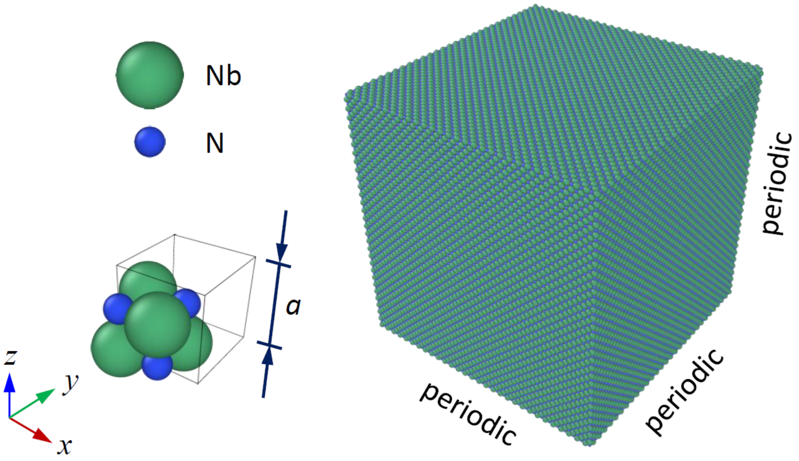


Figure S9: Schematic of the simulation supercell model used for the SED analysis. Left: the cubic NbN unit cell showing niobium (green) and nitrogen (blue) atoms. The unit cell side lenght is $a = 4.482262$ Å. Right: a supercell comprising $N_x \times N_y \times N_z = 30 \times 30 \times 30$ unit cells with periodic boundary conditions applied in all three spatial directions.

The SED spectrum is computed using the following expression [S2, S3]:

$$\Phi'(\boldsymbol{\kappa}, \omega) = \sum_{\alpha}^{3} \sum_{b}^{n} \left| \mu_0 \sum_{l}^{N} \int_{0}^{\tau_0} \dot{u}_\alpha \begin{pmatrix} l \\ b \end{pmatrix}; t) \, e^{\mathrm{i}\left[\boldsymbol{\kappa} \cdot \boldsymbol{r}_0 \begin{pmatrix} l \\ 0 \end{pmatrix} - wt\right]} \mathrm{d}t \right|^2, \tag{S1}$$

where $\dot{u}_\alpha$ is the $\alpha$-component of the velocity of the $b$th atom in the $l$th unit cell at time $t$, $\mu_0 = m_b/(4\pi\tau_0 N)$, $\tau_0$ is the total simulation time, $\boldsymbol{r}_0$ is the equilibrium position vector of the $l$th unit cell, and $n$ is the number of atoms per unit cell.

A schematic highlighting the high-symmetry points of the cubic NbN supercell is shown in Fig. S10. These high-symmetry points define the wave-vector paths used in the SED analysis. The wave-vector component along direction $\alpha$ is given by:

$$\kappa_\alpha = 2\pi j/(N_\alpha a), j = 0, 1, 2, ...N_\alpha/2, \alpha = x, y, z. \tag{S2}$$

The wave-vector resolution along each principal direction is given by $\Delta\kappa = 0.033\,(2\pi/a)$. We note that in Eq. (S1), the phonon frequencies can be obtained only for a discrete set of allowed wave vectors as determined by the size and periodicity of the supercell.

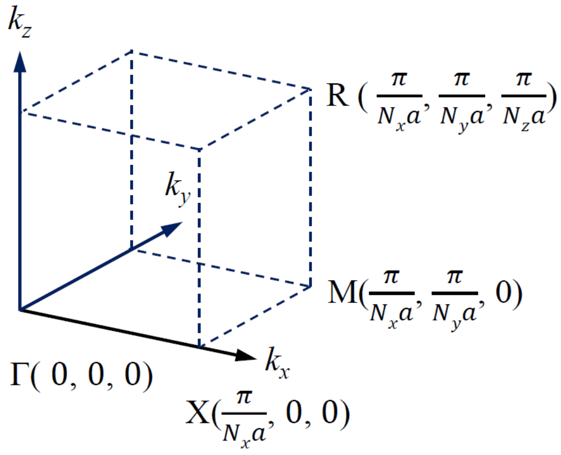


Figure S10: Schematic showing high-symmetry points that define the wave vector directions used in the SED calculations.

## References


S1 S. Plimpton, Fast parallel algorithms for short-range molecular dynamics, J. Comput. Phys. **117**, 1 (1995).

S2 J. Larkin, J. Turney, A. Massicotte, C. Amon, and A. McGaughey, Comparison and evaluation of spectral energy methods for predicting phonon properties, Journal of Computational and Theoretical Nanoscience **11**, 249 (2014).

S3 J. A. Thomas, J. E. Turney, R. M. Iutzi, C. H. Amon, and A. J. McGaughey, Predicting phonon dispersion relations and lifetimes from the spectral energy density, Phys. Rev. B **81**, 081411 (2010).
